# Supplementary material for: Physics Informed Deep Learning (Part II): Data-driven Discovery of Nonlinear Partial Differential Equations
Source: arXiv:1711.10566 source file (2017-11-28)
Supplement: Supplementary file 1 [file appendix.tex]

\section{Systematic studies}

\subsection{Continuous Time Models}

\subsubsection{Example (Burgers' Equation)}
As an example, let us consider the Burgers' equation. This equation arises in various areas of applied mathematics, including fluid mechanics, nonlinear acoustics, gas dynamics, and traffic flow \cite{basdevant1986spectral}. It is a fundamental partial differential equation and can be derived from the Navier-Stokes equations for the velocity field by dropping the pressure gradient term. 
% Burgers' equation, despite its relation to the much more complicated Navier-Stokes equations, does not exhibit turbulent behavior. 
For small values of the viscosity parameters, Burgers' equation can lead to shock formation that is notoriously hard to resolve by classical numerical methods. In one space dimension the Burger's equation along with Dirichlet boundary conditions reads as
\begin{eqnarray}\label{eq:Burgers}
&& u_t + u u_x - (0.01/\pi) u_{xx} = 0,\ \ \ x \in [-1,1],\ \ \ t \in [0,1],\\
&& u(0,x) = -\sin(\pi x),\nonumber\\
&& u(t,-1) = u(t,1) = 0.\nonumber
\end{eqnarray}
Let us define $f(t,x)$ to be given by
\[
f := u_t + u u_x - (0.01/\pi) u_{xx},
\]
and proceed by approximating $u(t,x)$ by a deep neural network. To highlight the simplicity in implementing this idea we have included a  Python code snippet using Tensorflow \cite{abadi2016tensorflow}; currently one of the most popular and well documented open source libraries for machine learning computations. To this end, $u(t,x)$ can be simply defined as
\begin{lstlisting}[language=Python]
def neural_net(H, weights, biases):
    for l in range(0,num_layers-2):
        W = weights[l]; b = biases[l]
        H = tf.tanh(tf.add(tf.matmul(H, W), b)) # tanh(HW + b)
    W = weights[-1]; b = biases[-1]
    H = tf.add(tf.matmul(H, W), b) # HW + b
    return H

def u(t, x):
    u = neural_net(tf.concat([t,x],1), weights, biases)
    return u
\end{lstlisting}
Correspondingly, the \emph{physic informed neural network} $f(t,x)$ takes the form
\begin{lstlisting}[language=Python]
def f(t, x):
    u = u(t, x)
    u_t = tf.gradients(u, t)[0]
    u_x = tf.gradients(u, x)[0]
    u_xx = tf.gradients(u_x, x)[0]
    f = u_t + u*u_x - (0.01/tf.pi)*u_xx
    return f
\end{lstlisting}
The shared parameters between the neural networks $u(t,x)$ and $f(t,x)$ can be learned by minimizing the mean squared error loss
\begin{equation}\label{eq:MSE_Burgers_CT_inference}
MSE = MSE_u + MSE_f,
\end{equation}
where
\[
MSE_u = \frac{1}{N_u}\sum_{i=1}^{N_u} |u(t^i_u,x_u^i) - u^i|^2,
\]
and
\[
MSE_f = \frac{1}{N_f}\sum_{i=1}^{N_f}|f(t_f^i,x_f^i)|^2.
\]
Here, $\{t_u^i, x_u^i, u^i\}_{i=1}^{N_u}$ denote the initial and boundary training data on $u(t,x)$ and $\{t_f^i, x_f^i\}_{i=1}^{N_f}$ specify the collocations points for $f(t,x)$. The loss $MSE_u$ corresponds to the initial and boundary data while $MSE_f$ enforces the structure imposed by equation \eqref{eq:Burgers} at a finite set of collocation points. 

In all benchmarks considered in this work, the total number of training data $N_u$ is relatively small (a few hundred up to a few thousand points), and we chose to optimize all loss functions using 
using L-BFGS; a quasi-Newton, full-batch gradient-based optimization algorithm \cite{liu1989limited}. For larger data-sets a more computationally efficient mini-batch setting can be readily employed using stochastic gradient descent and its modern variants \cite{goodfellow2016deep}. Despite the fact that this procedure is only guaranteed to converge to a local minimum, our empirical evidence indicates that, if the given partial differential equation is well-posed and its solution is unique, our method is capable of achieving good prediction accuracy given a sufficiently expressive neural network architecture and a sufficient number of collocation points $N_f$. 
This general observation will be quantified by specific sensitivity studies that accompany the numerical examples presented in the following.

Figure~\ref{fig:Burgers_CT_inference} summarizes our results for the 
data-driven solution of the Burgers equation. Specifically, given a set of $N_u = 100$ randomly distributed initial and boundary data, we learn the latent solution $u(t,x)$ by training all ? parameters of a 9-layer deep neural network using the mean squared error loss of \eqref{eq:MSE_Burgers_CT_inference}. Each hidden layer contained $20$ neurons and a hyperbolic tangent activation function. In general, the neural network should be given sufficient approximation capacity in order to accommodate the anticipated complexity of $u(t,x)$. However, in this example, our choice aims to highlight the robustness of the proposed method with respect to the well known issue of over-fitting. Specifically, the term in $MSE_f$ in equation \eqref{eq:MSE_Burgers_CT_inference} acts as a regularization mechanism that penalizes solutions that do not satisfy equation \eqref{eq:Burgers}. Therefore, a key property of {\em physics informed neural networks} is that they can be effectively trained using small data sets; a setting often encountered in the study of physical systems for which the cost of data acquisition may be prohibitive. 

The top panel of Figure~\ref{fig:Burgers_CT_inference} shows the predicted spatio-temporal solution $u(t,x)$, along with the locations of the initial and boundary training data. We must underline that, unlike any classical numerical method for solving partial differential equations, this prediction is obtained without any sort of discretization of the spatio-temporal domain. The exact solution for this problem is analytically available \cite{basdevant1986spectral}, and the resulting prediction error is measured at $6.7 \cdot 10^{-4}$ in the relative $\mathbb{L}_2$-norm. Note that this error is about two orders of magnitude lower than the one reported in our previous work on data-driven solution of partial differential equation using Gaussian processes \cite{raissi2017numerical}. A more detailed assessment of the predicted solution is presented in the bottom panel of Figure~\ref{fig:Burgers_CT_inference}. In particular, we present a comparison between the exact and the predicted solutions at different time instants $t=0.25,0.50,0.75$.
Using only a handful of initial data, the {\em physics informed neural network} can accurately capture the intricate nonlinear behavior of the Burgers equation that leads to the development of sharp internal layer around $t = 0.4$. The latter is notoriously hard to accurately resolve with classical numerical methods and requires a laborious spatio-temporal discretization of Eq.~\eqref{eq:Burgers}.

\begin{figure}
\includegraphics[width = 1.0\textwidth]{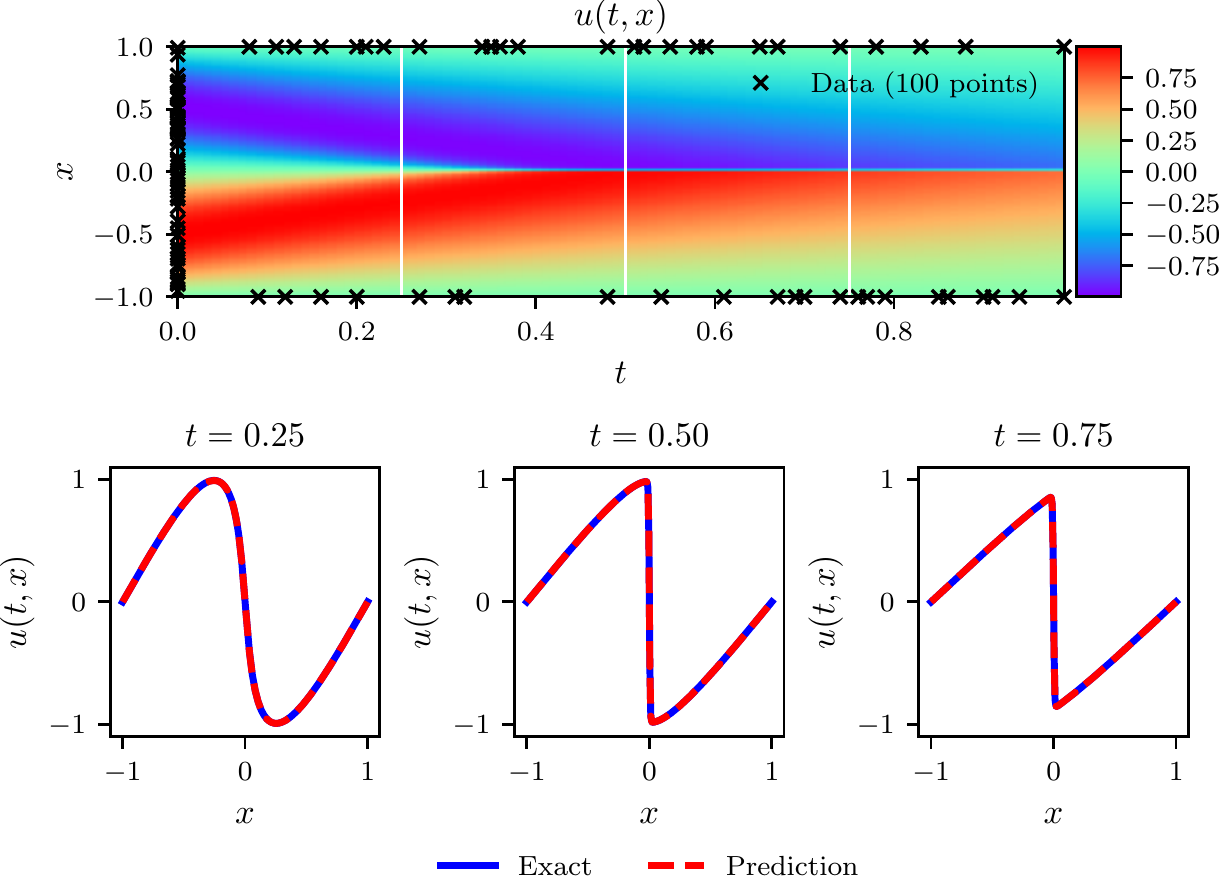}
\caption{{\em Burgers equation:} {\it Top:} Predicted solution $u(t,x)$ along with the initial and boundary training data. In addition we are using 10,000 collocation points generated using a Latin Hypercube Sampling strategy. {\it Bottom:} Comparison of the predicted and exact solutions corresponding to  the three temporal snapshots depicted by the dashed vertical lines in the top panel. The relative $\mathbb{L}_{2}$ error for this case is $6.7 \cdot 10^{-4}$, with model training taking approximately 60 seconds on one NVIDIA Titan X GPU.}
\label{fig:Burgers_CT_inference}
\end{figure}

To further analyze the performance of our method, we have performed systematic study to quantify its predictive accuracy for different number of training and collocation points, as well as for different neural network architectures. In Table~\ref{tab:Burgers_CT_inference_1} we report the resulting relative $\mathbb{L}_{2}$ error for different number of initial and boundary training data $N_u$ and different number of collocation points $N_f$, while keeping the 9-layer network architecture fixed. The general trend shows increased prediction accuracy as the total number of training data $N_u$ is increased, given a sufficient number of collocation points $N_f$. This observation highlights the key strength of {\em physics informed neural networks}: by encoding the structure of the underlying physical law through the collocation points $N_f$ one can obtain a more accurate and data-efficient learning algorithm. 
\footnote{Note that the case $N_f = 0$ corresponds to a standard neural network model, i.e. a neural network that does not take into account the underlying governing equation.}
Finally, Table~\ref{tab:Burgers_CT_inference_2} shows the resulting relative $\mathbb{L}_{2}$ for different number of hidden layers, and different number of neurons per layer, while the total number of training and collocation points is kept fixed to 
$N_u = 100$ and $N_f=10000$, respectively. As expected, we observe that as the number of layers and neurons is increased (hence the capacity of the neural network to approximate more complex functions), the predictive accuracy is increased.

\begin{table}
\label{tab:Burgers_CT_inference_1}
\centering
\begin{tabular}{|l||cccccc|} 
\hline
\diagbox{$N_u$}{$N_f$} & 2000 & 4000 & 6000 & 7000 & 8000 & 10000 \\ \hline\hline
20 & 2.9e-01 & 4.4e-01 & 8.9e-01 & 1.2e+00 & 9.9e-02 & 4.2e-02 \\ 
40 & 6.5e-02 & 1.1e-02 & 5.0e-01 & 9.6e-03 & 4.6e-01 & 7.5e-02 \\ 
60 & 3.6e-01 & 1.2e-02 & 1.7e-01 & 5.9e-03 & 1.9e-03 & 8.2e-03 \\ 
80 & 5.5e-03 & 1.0e-03 & 3.2e-03 & 7.8e-03 & 4.9e-02 & 4.5e-03 \\ 
100 & 6.6e-02 & 2.7e-01 & 7.2e-03 & 6.8e-04 & 2.2e-03 & 6.7e-04 \\ 
200 & 1.5e-01 & 2.3e-03 & 8.2e-04 & 8.9e-04 & 6.1e-04 & 4.9e-04 \\ \hline
\end{tabular}
\caption{{\em Burgers' equation:} Relative $\mathbb{L}_{2}$ error between the predicted and the exact solution $u(t,x)$ for different number of initial and boundary training data $N_u$, and different number of collocation points $N_f$. Here, the network architecture is fixed to 9 layers with 20 neurons per hidden layer.}
\end{table}

\begin{table}
\label{tab:Burgers_CT_inference_2}
\centering
\begin{tabular}{|c||ccc|} 
\hline
\diagbox{Layers}{Neurons} & 10 & 20 & 40  \\ \hline\hline
2 & 7.4e-02 & 5.3e-02 & 1.0e-01 \\ 
4 & 3.0e-03 & 9.4e-04 & 6.4e-04 \\ 
6 & 9.6e-03 & 1.3e-03 & 6.1e-04 \\ 
8 & 2.5e-03 & 9.6e-04 & 5.6e-04 \\ \hline
\end{tabular}
\caption{{\em Burgers' equation:} Relative $\mathbb{L}_{2}$ error between the predicted and the exact solution $u(t,x)$ for different number of hidden layers, and different number of neurons per layer. Here, the total number of training and collocation points is fixed to 
$N_u = 100$ and $N_f=10000$, respectively.}
\end{table}

\subsection{Discrete Time Models}

\subsubsection{Example (Burgers' Equation)}
To highlight the key features of the discrete time representation we revisit the problem of data-driven solution of the Burgers' equation. The nonlinear operator in equation \eqref{eq:RungeKutta_inference_rearranged} is given by
\[
\mathcal{N}[u^{n+c_j}] = u^{n+c_j} u^{n+c_j}_x - (0.01/\pi)u^{n+c_j}_{xx}
\]
and the shared parameters of the neural networks \eqref{eq:RungeKutta_PU_prior_inference} and \eqref{eq:RungeKutta_PI_prior_inference} can be learned by minimizing the sum of squared errors
\[
SSE = SSE_n + SSE_b
\]
where
\[
SSE_n = \sum_{j=1}^q \sum_{i=1}^{N_n} |u^n_j(x^{n,i}) - u^{n,i}|^2,
\]
and
\[
SSE_b = \sum_{i=1}^q \left(|u^{n+c_i}(-1)|^2 + |u^{n+c_i}(1)|^2\right) + |u^{n+1}(-1)|^2 + |u^{n+1}(1)|^2.
\]
Here, $\{x^{n,i}, u^{n,i}\}_{i=1}^{N_n}$ corresponds to the data at time $t^n$.

The Runge-Kutta scheme now allows us to infer the latent solution $u(t,x)$ in a sequential fashion. Starting from initial data $\{x^{n,i}, u^{n,i}\}_{i=1}^{N_n}$ at time $t^n$ and data at the domain boundaries $x = -1$ and $x = 1$ at time $t^{n+1}$, we can use the aforementioned loss functions to train the networks of \eqref{eq:RungeKutta_PU_prior_inference}, \eqref{eq:RungeKutta_PI_prior_inference}, and predict the solution at time $t^{n+1}$. A Runge-Kutta time-stepping scheme would then use this prediction as initial data for the next step and proceed to train again and predict $u(t^{n+2},x)$, $u(t^{n+3},x)$, etc., one step at a time. 

In classical numerical analysis, these steps are usually confined to be small due to stability constraints for explicit schemes or computational complexity constrains for implicit formulations \cite{iserles2009first}. 
These constraints become more severe as the total number of Runge-Kutta stages $q$ is increased, and, for most problems of practical interest, one needs to take thousands to millions of such steps until the solution is resolved up to a desired final time. In sharp contrast to classical methods, here we can employ implicit Runge-Kutta schemes with an arbitrarily large number of stages at effectively no extra cost. 
\footnote{To be precise, it is only the number of parameters in the last layer of the neural network that increases linearly with the total number of stages.}
This enables us to take very large time steps while retaining stability and high predictive accuracy, therefore allowing us to resolve the entire spatio-temporal solution in a single step.

The result of applying this process to the Burgers' equation is presented in Figure~\ref{fig:Burgers_DT_inference}. For illustration purposes, we start with a set of $N_n=250$ initial data at $t = 0.1$, and employ a {\em physics informed neural network} induced by an implicit Runge-Kutta scheme with 500 stages to predict the solution at time $t=0.9$ in a single step. The theoretical error estimates for this scheme predict a temporal error accumulation of $\mathcal{O}(\Delta{t}^{2q})$ \cite{iserles2009first}, which in our case translates into an error way below machine precision, i.e., $\Delta{t}^q = 0.8^{1000} \approx 10^{-97}$. To our knowledge, this is the first time that an implicit Runge-Kutta scheme of that high-order has ever been used. Remarkably, starting from a smooth initial data at $t=0.1$ we can predict the nearly discontinuous solution at $t=0.9$ in a single time-step with a relative $\mathbb{L}_{2}$ error of $6.7 \cdot 10^{-4}$. This error is two orders of magnitude lower that the one reported in \cite{raissi2017numerical}, and it is entirely attributed to the neural network's capacity to approximate $u(t,x)$, as well as to the degree that the sum of squared errors loss allows interpolation of the training data. The network architecture used here consists of 4 layers with 50 neurons in each hidden layer. 

\begin{figure}
\includegraphics[width = 1.0\textwidth]{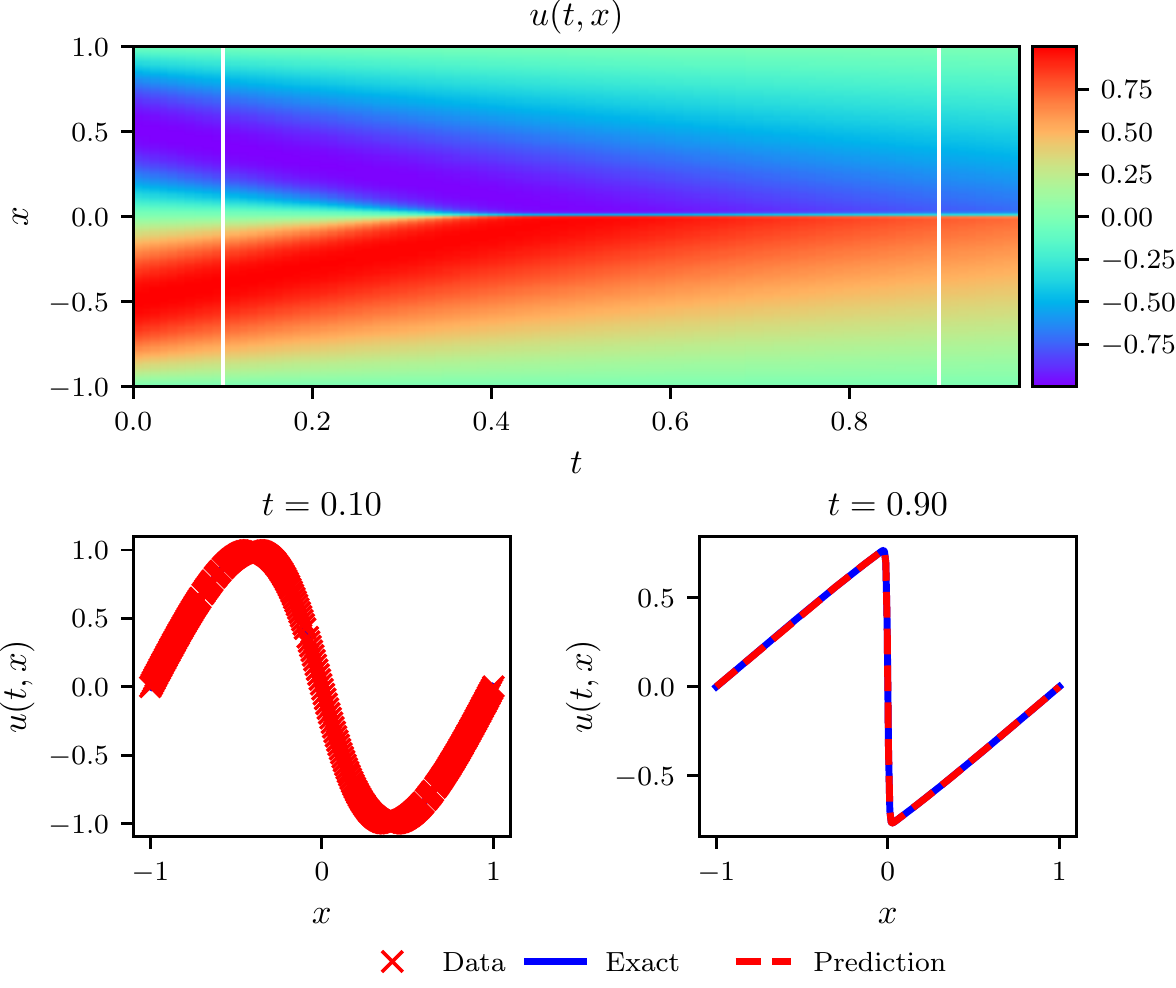}
\caption{{\em Burgers equation:} {\it Top:} Solution $u(t,x)$ along with the location of the initial training snapshot at $t=0.1$ and the final prediction snapshot at $t=0.9$. {\it Bottom:} Initial training data and final prediction at the snapshots depicted by the white vertical lines in the top panel. The relative $\mathbb{L}_{2}$ error for this case is $6.7 \cdot 10^{-4}$, with model training taking approximately 60 seconds on one NVIDIA Titan X GPU.}
\label{fig:Burgers_DT_inference}
\end{figure}

A detailed systematic study to quantify the effect of different network architectures is presented in Table~\ref{tab:Burgers_DT_inference_2}. By keeping the number of Runge-Kutta stages fixed to 500 and the time-step size to $\Delta{t}=0.8$, we have varied the number of hidden layers and the number of neurons per layer, and monitored the resulting relative $\mathbb{L}_{2}$ error for the predicted solution at time $t=0.9$. Evidently, as the neural network capacity is increased the predictive accuracy is enhanced.

\begin{table}
\label{tab:Burgers_DT_inference_2}
\centering
\begin{tabular}{|c||ccc|} 
\hline
\diagbox{Layers}{Neurons} & 10 & 25 & 50  \\ \hline\hline
1 & 4.1e-02 & 4.1e-02 & 1.5e-01 \\
2 & 2.7e-03 & 5.0e-03 & 2.4e-03 \\
3 & 3.6e-03 & 1.9e-03 & 9.5e-04 \\ \hline
\end{tabular}
\caption{{\em Burgers' equation:} Relative final prediction error measure in the $\mathbb{L}_{2}$ norm for different number of hidden layers and neurons in each layer. Here, the number of Runge-Kutta stages is fixed to 500 and the time-step size to $\Delta{t}=0.8$.}
\end{table}

The key parameters controlling the performance of our discrete time algorithm are the total number of Runge-Kutta stages $q$ and the time-step size $\Delta{t}$. In Table~\ref{tab:Burgers_DT_inference_1} we summarize the results of an extensive systematic study where we fix the network architecture to 4 hidden layers with 50 neurons per layer, and vary the number of Runge-Kutta stages $q$ and the time-step size $\Delta{t}$. Specifically, we see how cases with low numbers of stages fail to yield accurate results when the time-step size is large. For instance, the case $q=1$ corresponding to the classical trapezoidal rule, and the case $q=2$ corresponding to the $4^{\text{th}}$-order Gauss-Legendre method, cannot retain their predictive accuracy for time-steps larger than 0.2, thus mandating a solution strategy with multiple time-steps of small size. On the other hand, the ability to push the number of Runge-Kutta stages to 32 and even higher allows us to take very large time steps, and effectively resolve the solution in a single step without sacrificing the accuracy of our predictions. Moreover, numerical stability is not sacrificed either as implicit Runge-Kutta is the only family of time-stepping schemes that remain A-stable regardless for their order, thus constituting them ideal for stiff problems \cite{iserles2009first}. These properties are previously unheard-of for an algorithm of such implementation simplicity, and illustrate one of the key highlights of our discrete time approach.

\begin{table}
\label{tab:Burgers_DT_inference_1}
\centering
\begin{tabular}{|l||cccc|} 
\hline
\diagbox{$q$}{$\Delta{t}$} & 0.2 & 0.4 & 0.6 & 0.8 \\ \hline\hline
1 & 3.5e-02 & 1.1e-01 & 2.3e-01 & 3.8e-01 \\
2 & 5.4e-03 & 5.1e-02 & 9.3e-02 & 2.2e-01 \\
4 & 1.2e-03 & 1.5e-02 & 3.6e-02 & 5.4e-02 \\
8 & 6.7e-04 & 1.8e-03 & 8.7e-03 & 5.8e-02 \\
16 & 5.1e-04 & 7.6e-02 & 8.4e-04 & 1.1e-03 \\
32 & 7.4e-04 & 5.2e-04 & 4.2e-04 & 7.0e-04 \\
64 & 4.5e-04 & 4.8e-04 & 1.2e-03 & 7.8e-04 \\
100 & 5.1e-04 & 5.7e-04 & 1.8e-02 & 1.2e-03 \\
500 & 4.1e-04 & 3.8e-04 & 4.2e-04 & 8.2e-04 \\ \hline
\end{tabular}
\caption{{\em Burgers' equation:} Relative final prediction error measure in the $\mathbb{L}_{2}$ norm for different number of Runge-Kutta stages $q$ and time-step sizes $\Delta{t}$. Here, the network architecture is fixed to 4 hidden layers with 50 neurons in each layer.}
\end{table}

\subsection{Continuous Time Models}

\subsubsection{Example (Burgers' Equation)}
As a first example, let us again consider the Burgers' equation. In one space dimension the equation reads as
\begin{eqnarray}
&& u_t + \lambda_1 u u_x - \lambda_2 u_{xx} = 0
\end{eqnarray}
Let us define $f(t,x)$ to be given by
\[
f := u_t + \lambda_1 u u_x - \lambda_2 u_{xx},
\]
and proceed by approximating $u(t,x)$ by a deep neural network. This will result in the \emph{physics informed neural network} $f(t,x)$. The shared parameters of the neural networks $u(t,x)$ and $f(t,x)$ along with the parameters $\lambda = (\lambda_1, \lambda_2)$ of the differential operator can be learned by minimizing the mean squared error loss
\begin{equation}\label{eq:MSE_Burgers_CT_inference}
MSE = MSE_u + MSE_f,
\end{equation}
where
\[
MSE_u = \frac{1}{N}\sum_{i=1}^{N} |u(t^i_u,x_u^i) - u^i|^2,
\]
and
\[
MSE_f = \frac{1}{N}\sum_{i=1}^{N}|f(t_f^i,x_f^i)|^2.
\]
Here, $\{t_u^i, x_u^i, u^i\}_{i=1}^{N}$ denote the training data on $u(t,x)$. The loss $MSE_u$ corresponds to the training data on $u(t,x)$ while $MSE_f$ enforces the structure imposed by equation \eqref{eq:Burgers} at a finite set of collocation points, whose number and location is taken to be the same with the training data.

To illustrate the effectiveness of our approach we have created a training data-set by randomly generating $N = 2000$ points across the entire spatio-temporal domain from the exact solution corresponding to $\lambda_1 = 1.0$ and $\lambda_2 = 0.01/\pi$. The locations of the training points are illustrated in the top panel of Figure~\ref{fig:Burgers_CT_identification}.
This data-set is then used to train a 9-layer deep neural network with 20 neurons per hidden layer by minimizing the mean square error loss of \eqref{eq:MSE_Burgers_CT_inference} using the L-BFGS optimizer \cite{liu1989limited}. Upon training, the networks parameters are calibrated to predict the entire solution $u(t,x)$, as well as the unknown parameters $\lambda = (\lambda_1, \lambda_2)$ that define the underlying dynamics. A visual assessment of the predictive accuracy of the {\em physics informed neural network} is given at the middle and bottom panels of Figure~\ref{fig:Burgers_CT_identification}. The network is able to identify the underlying partial differential equation with remarkable accuracy, even in the case which the scattered training data is corrupted with 1\% uncorrelated noise.

\begin{figure}
\includegraphics[width = 1.0\textwidth]{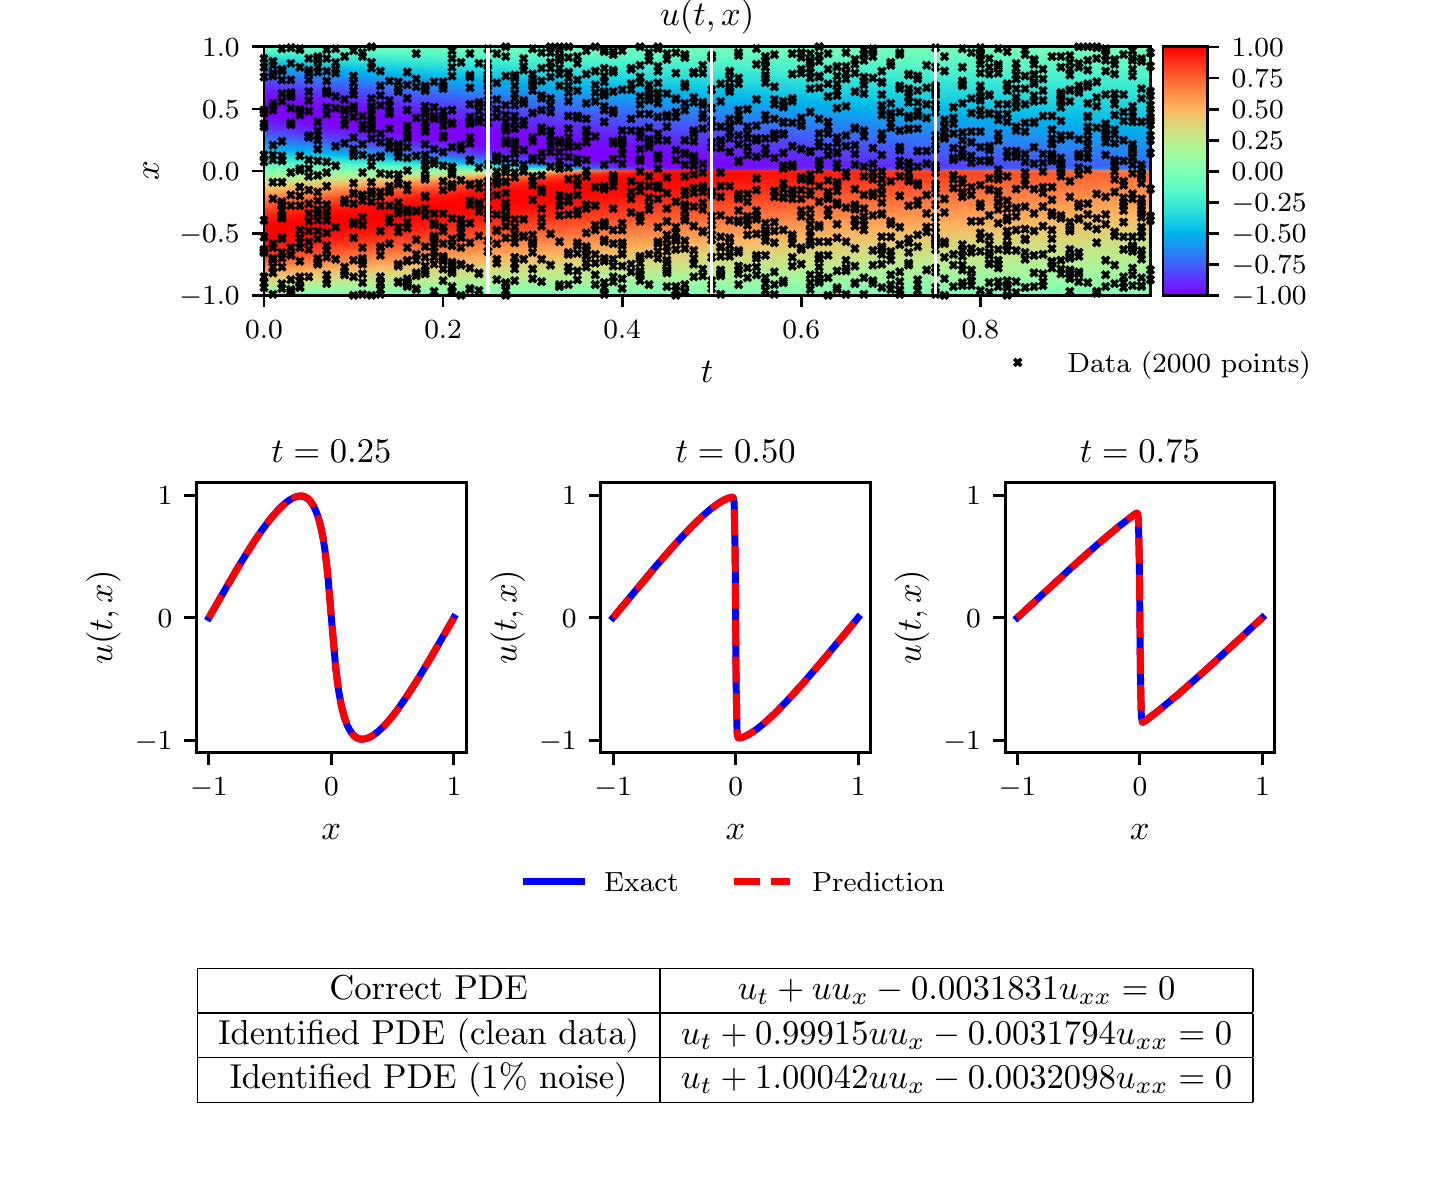}
\caption{{\em Burgers equation:} {\it Top:} Predicted solution $u(t,x)$ along with the training data. {\it Middle:} Comparison of the predicted and exact solutions corresponding to  the three temporal snapshots depicted by the dashed vertical lines in the top panel. {\it Bottom:} Correct partial differential equation along with the identified one obtained by learning $\lambda_1, \lambda_2$.}
\label{fig:Burgers_CT_identification}
\end{figure}

To further scrutinize the performance of our algorithm we have performed a systematic study with respect to the total number of training data, the noise corruption levels, and the neural network architecture. The results as summarized in Tables~\ref{tab:Burgers_CT_identification_1} and~\ref{tab:Burgers_CT_identification_2}. The key observation here is that the proposed methodology appears to be very robust with respect to noise levels in the data, and yield a reasonable identification accuracy even for noise corruption up to 10\%. This enhanced robustness seems to greatly outperform competing approaches using Gaussian process regression as previously reported in \cite{raissi2017hidden}, as well as approaches relying on sparse regression that require relatively clean data for accurately computing numerical gradients \cite{brunton2016discovering}.

\begin{table}
\label{tab:Burgers_CT_identification_1}
\centering
\begin{tabular}{|l||cccc||cccc|} \hline
& \multicolumn{4}{c||}{\% error in $\lambda_1$} & \multicolumn{4}{c|} {\% error in $\lambda_2$} \\ \hline
\diagbox{$N_u$}{noise} & 0\% & 1\% & 5\% & 10\% & 0\% & 1\% & 5\% & 10\% \\ \hline\hline
500 &  0.131 & 0.518 & 0.118 & 1.319 & 13.885 & 0.483 & 1.708 & 4.058 \\
1000 & 0.186 & 0.533 & 0.157 & 1.869 & 3.719 & 8.262 & 3.481 & 14.544 \\
1500 & 0.432 & 0.033 & 0.706 & 0.725 & 3.093 & 1.423 & 0.502 & 3.156 \\
2000 & 0.096 & 0.039 & 0.190 & 0.101 & 0.469 & 0.008 & 6.216 & 6.391 \\ \hline
\end{tabular}
\caption{{\em Burgers' equation:} Percentage error in the identified parameters $\lambda_1$ and $\lambda_2$ for different number of training data $N_u$ corrupted by different noise levels. Here, the neural network architecture is kept fixed to 9 layers and 20 neurons per layer.}
\end{table}

\begin{table}
\label{tab:Burgers_CT_identification_2}
\centering
\begin{tabular}{|c||ccc||ccc|} \hline
& \multicolumn{3}{c||}{\% error in $\lambda_1$} & \multicolumn{3}{c|} {\% error in $\lambda_2$} \\ \hline
\diagbox{Layers}{Neurons} & 10 & 20 & 40 & 10 & 20 & 40 \\ \hline\hline
2 & $11.696$ & $2.837$ & $1.679$ & $103.919$ & $67.055$ & $49.186$ \\
4 & $0.332$ & $0.109$ & $0.428$ & $4.721$ & $1.234$ & $6.170$ \\
6 & $0.668$ & $0.629$ & $0.118$ & $3.144$ & $3.123$ & $1.158$ \\
8 & $0.414$ & $0.141$ & $0.266$ & $8.459$ & $1.902$ & $1.552$ \\ \hline
\end{tabular}
\caption{{\em Burgers' equation:} Percentage error in the identified parameters $\lambda_1$ and $\lambda_2$ for different number of hidden layers and neurons per layer. Here, the training data is considered to be noise-free and fixed to $N = 2000$.}
\end{table}

\subsection{Discrete Time Models}

\subsubsection{Example (Burgers' Equation)}
Let us again illustrate the key features of this method through the lens of the Burgers' equation. Recall the equation's form
\begin{equation}\label{eq:Burgers_DT_identification}
u_t + \lambda_1 u u_x - \lambda_2 u_xx = 0,
\end{equation}
and notice that the nonlinear operator in equation \eqref{eq:RungeKutta_identification_rearranged} is given by
\[
\mathcal{N}[u^{n+c_j}] = \lambda_1 u^{n+c_j} u^{n+c_j}_x - \lambda_2 u^{n+c_j}_{xx}.
\]
Given merely two training data snapshots, the shared parameters of the neural networks along with the parameters $\lambda = (\lambda_1, \lambda_2)$ can be learned by minimizing the sum of squared errors \eqref{eq:SSE_identification}. Here, we have created a training data-set comprising of $N_n=199$ and $N_{n+1}=201$ spatial points by randomly sampling the exact solution at time instants $t^n=0.1$ and $t^{n+1}=0.9$, respectively. The training data, along with the predictions of the trained network, are shown in the top and middle panel of Figure~\ref{fig:Burgers_DT_identification}. The neural network architecture used here includes 4 hidden layers with 50 neurons each, while the number of Runge-Kutta stages is empirically chosen to yield a temporal error accumulation of the order of machine precision $\epsilon$ by setting 
\footnote{This is motivated by the theoretical error estimates for implicit Runge-Kutta schemes suggesting a truncation error of $\mathcal{O}(\Delta{t}^{2q})$ \cite{iserles2009first}.}
\begin{equation}\label{eq:Runge-Kutta_stages}
q = 0.5\log{\epsilon}/\log(\Delta{t}),
\end{equation}
where the time-step for this example is $\Delta{t}=0.8$. The bottom panel of Figure~\ref{fig:Burgers_DT_identification} summarizes the identified parameters $\lambda = (\lambda_1, \lambda_2)$ for the cases of noise-free data, as well as noisy data with 1\% of uncorrelated noise corruption. For both cases, the proposed algorithm is able to learn the correct parameter values $\lambda_1=1.0$ and  $\lambda_2=0.01/\pi$ with remarkable accuracy, despite the fact that the two data snapshots used for training are very far apart, and potentially describe different regimes of the underlying dynamics.

\begin{figure}
\includegraphics[width = 1.0\textwidth]{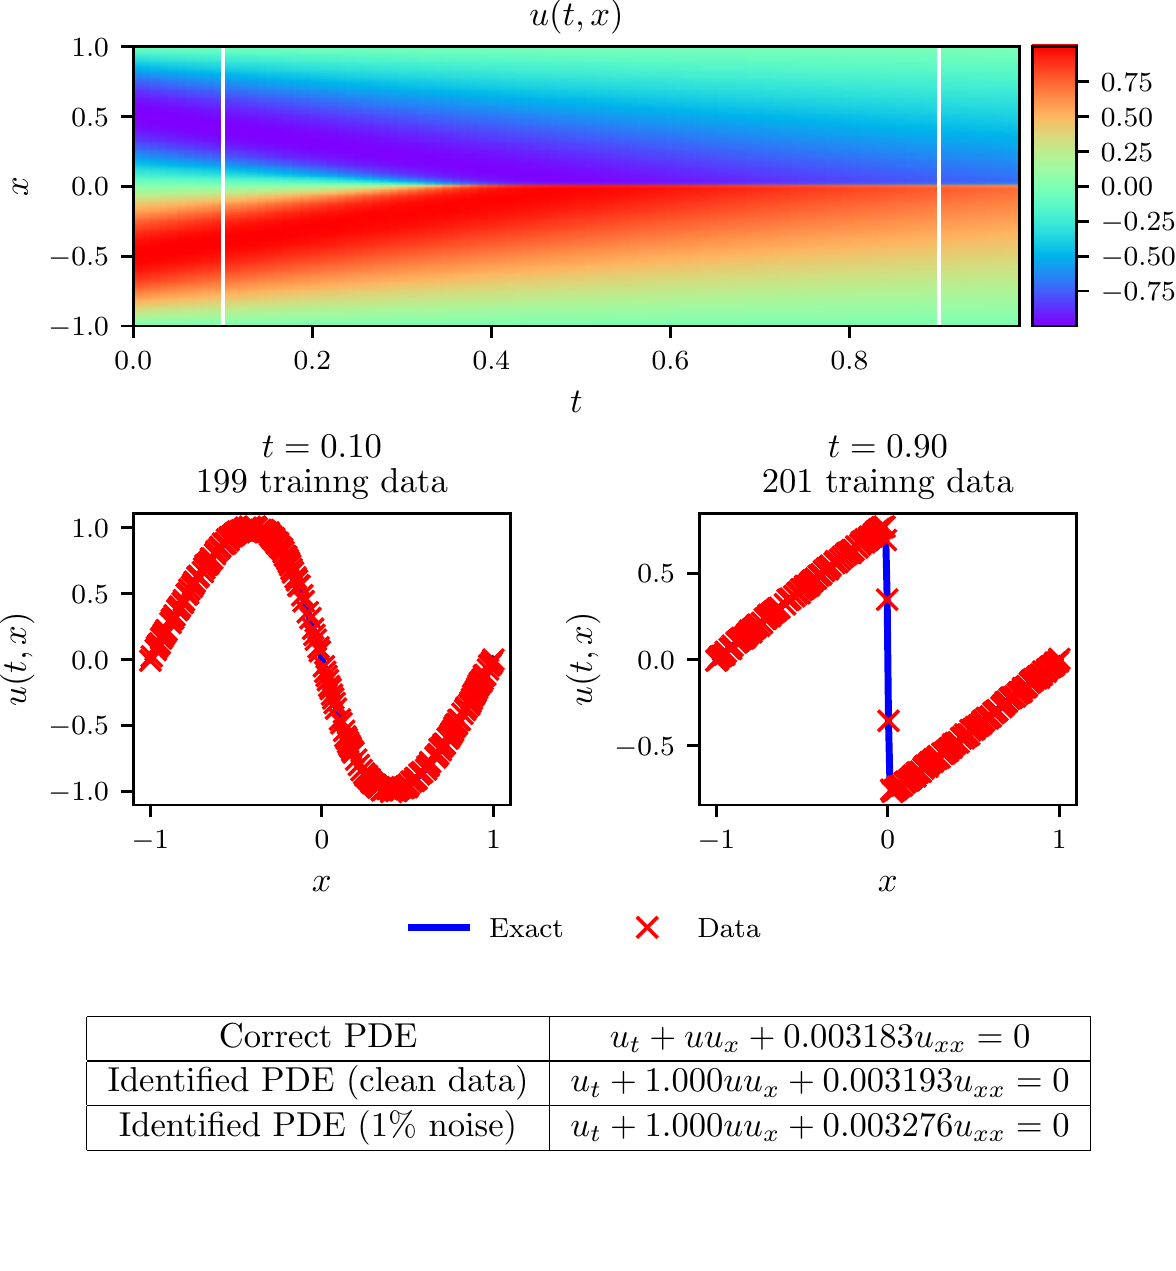}
\caption{{\em Burgers equation:} {\it Top:} Predicted solution $u(t,x)$ along with the temporal locations of the two training snapshots. {\it Middle:} Training data and exact solution corresponding to  the two temporal snapshots depicted by the dashed vertical lines in the top panel. {\it Bottom:} Correct partial differential equation along with the identified one obtained by learning $\lambda_1, \lambda_2$.}
\label{fig:Burgers_DT_identification}
\end{figure}

A further sensitivity analysis is performed to quantify the accuracy of our predictions with respect to the gap between the training snapshots $\Delta{t}$, the noise levels in the training data, and the {\em physics informed neural network} architecture. As shown in Table~\ref{tab:Burgers_DT_identification_1}, the proposed algorithm is quite robust to both $\Delta{t}$ and the noise corruption levels, and it consistently returns reasonable estimates for the unknown parameters. This robustness is mainly attributed to the flexibility of the underlying implicit Runge-Kutta scheme to admit an arbitrarily high number of stages, allowing the data snapshots to be very far apart in time, while not compromising the accuracy with which the nonlinear dynamics of Eq.~\eqref{eq:Burgers_DT_identification} are resolved. This is the key highlight of our discrete time formulation for identification problems, setting apart from competing approaches \cite{raissi2017hidden,brunton2016discovering}. Lastly, Table~\ref{tab:Burgers_DT_identification_2} presents the percentage error in the identified parameters, demonstrating the robustness of our estimates with respect to the underlying neural network architecture.

\begin{table}
\label{tab:Burgers_DT_identification_1}
\centering
\begin{tabular}{|l||cccc||cccc|} \hline
& \multicolumn{4}{c||}{\% error in $\lambda_1$} & \multicolumn{4}{c|} {\% error in $\lambda_2$} \\ \hline
\diagbox{$\Delta{t}$}{noise} & 0\% & 1\% & 5\% & 10\% & 0\% & 1\% & 5\% & 10\% \\ \hline\hline
0.2 & $0.002$ & $0.435$ & $6.073$ & $3.273$ & $0.151$ & $4.982$ & $59.314$ & $83.969$ \\
0.4 & $0.001$ & $0.119$ & $1.679$ & $2.985$ & $0.088$ & $2.816$ & $8.396$ & $8.377$ \\
0.6 & $0.002$ & $0.064$ & $2.096$ & $1.383$ & $0.090$ & $0.068$ & $3.493$ & $24.321$ \\
0.8 & $0.010$ & $0.221$ & $0.097$ & $1.233$ & $1.918$ & $3.215$ & $13.479$ & $1.621$ \\ \hline
\end{tabular}
\caption{{\em Burgers' equation:} Percentage error in the identified parameters $\lambda_1$ and $\lambda_2$ for different gap size $\Delta{t}$ between two different snapshots and for different noise levels.}
\end{table}

\begin{table}
\label{tab:Burgers_DT_identification_2}
\centering
\begin{tabular}{|c||ccc||ccc|} \hline
& \multicolumn{3}{c||}{\% error in $\lambda_1$} & \multicolumn{3}{c|} {\% error in $\lambda_2$} \\ \hline
\diagbox{Layers}{Neurons} & 10 & 25 & 50 & 10 & 25 & 50 \\ \hline\hline
1 & $1.868$ & $4.868$ & $1.960$ & $180.373$ & $237.463$ & $123.539$ \\
2 & $0.443$ & $0.037$ & $0.015$ & $29.474$ & $2.676$ & $1.561$ \\
3 & $0.123$ & $0.012$ & $0.004$ & $7.991$ & $1.906$ & $0.586$ \\
4 & $0.012$ & $0.020$ & $0.011$ & $1.125$ & $4.448$ & $2.014$ \\ \hline
\end{tabular}
\caption{{\em Burgers' equation:} Percentage error in the identified parameters $\lambda_1$ and $\lambda_2$ for different number of hidden layers and neurons in each layer.}
\end{table}
